# Supplementary material for: CUPID: A Real-Time Session-Based Reciprocal Recommendation System for a One-on-One Social Discovery Platform
Source: arXiv:2410.18087 source file (2024-10-08)
Supplement: Supplementary file 1 [file A_appendix.tex]

\input{Tables/2_delayed_session_representation}

\section{Appendix}\label{sec:a_appendix}

\subsection{Experiment Details}

In our study, we employed Wide\&Deep to produce user feature representations $\mathbf{e}^u$ and matching history representations $\mathbf{e}^m$. 
The deep component of Wide\&Deep is composed of hidden layers with a size of [512, 256] and ReLU activations. 
The user feature representations and the matching history representations produced by the hidden layers have a dimension of 768. 
The session representations $\mathbf{e}^s$ also have a dimension of 768.
For user session modeling, we utilize a causal Transformer in GPT-2~\cite{radford2019language} and specifically use the bottom four layers of the original model. 
The maximum number of matching histories in user sessions is 128, and the dimension of the final user representations $\Bar{\mathbf{e}}$ after linear projection is 64. 
We implement our recommendation system using PyTorch and it is trained using the AdamW optimizer~\cite{loshchilov2019decoupled} with a learning rate of 1\textit{e}-4 and the ReduceLROnPlateau scheduler. The training of \textsc{Cupid} is conducted for three days using eight DGX A100 (40GB) GPUs. 
To evaluate the performance of each model, we trained it until it converged and reported the average performance across all matching histories.

\subsection{Effect of Delayed Session Representation}\label{subsec:5_5_effect_of_delayed_session_representation}

In Section~\ref{subsec:4_2_async_session_embedding_layer}, note that the session representation may not be updated yet before the session representation lookup occurs because the computation of the session representation may not be finished until a new match is requested.
We refer to the lookuped session representation in this scenario as a \textit{delayed} session representation.
Now, we will analyze the performance changes observed due to the delayed session representation .
Session representation $\mathbf{e}^s$ in the actual deployment environment may not always be updated with the recent matching histories. 
Suppose a user requests a new match before the computation of the user session representation is complete. 
In that case, the session representation looked up by our recommendation system to predict the chat duration would be the delayed one, computed from matching history without the last few matches. 
We simulate such an actual deployment environment to observe performance changes caused by these delayed session representations. 
Assuming that the delay in representation calculation takes $t'$ milliseconds, we predict the chat duration of users in the matching pool $\mathcal{U}^{(t)}$ at time $t$ using delayed session representation computed using the matching histories ended before $(t-t')$. 
The results of this experiment are summarized in Table~\ref{tab:2_delayed_session_representation}.

We have made two noteworthy observations regarding our model's performance. 
Firstly, we observe that the model's prediction performance slightly decreases as the delay time increases. 
However, this delay is a result of our system design, which decouples user session modeling from the synchronous matching pipeline. 
Without this delay, the slow computation for the user session modeling would act as a bottleneck, increasing latency significantly, as described in the following subsection. 
We believe that the slight decrease in prediction performance is an acceptable tradeoff to ensure low latency recommendation. 
Secondly, even with the performance drop caused by the delayed session representations, our models still outperform the Wide\&Deep-S baseline by a large margin in all cases, while showing similar latency. 
This indicates that our system design, with decoupled user session modeling, offers the best tradeoff between latency and prediction performance.
